# Supplementary material for: ScatterShot: Interactive In-context Example Curation for Text Transformation
Source: arXiv:2302.07346 source file (2023-02-14)
Supplement: Supplementary file 1 [file clusters.tex]

\section{Clustering for \qa}
\label{appendix:qa_cluster}

\begin{figure*}[h]
\centering
\includegraphics[trim={0cm 18cm 16cm 0cm}, clip,width=1\linewidth]{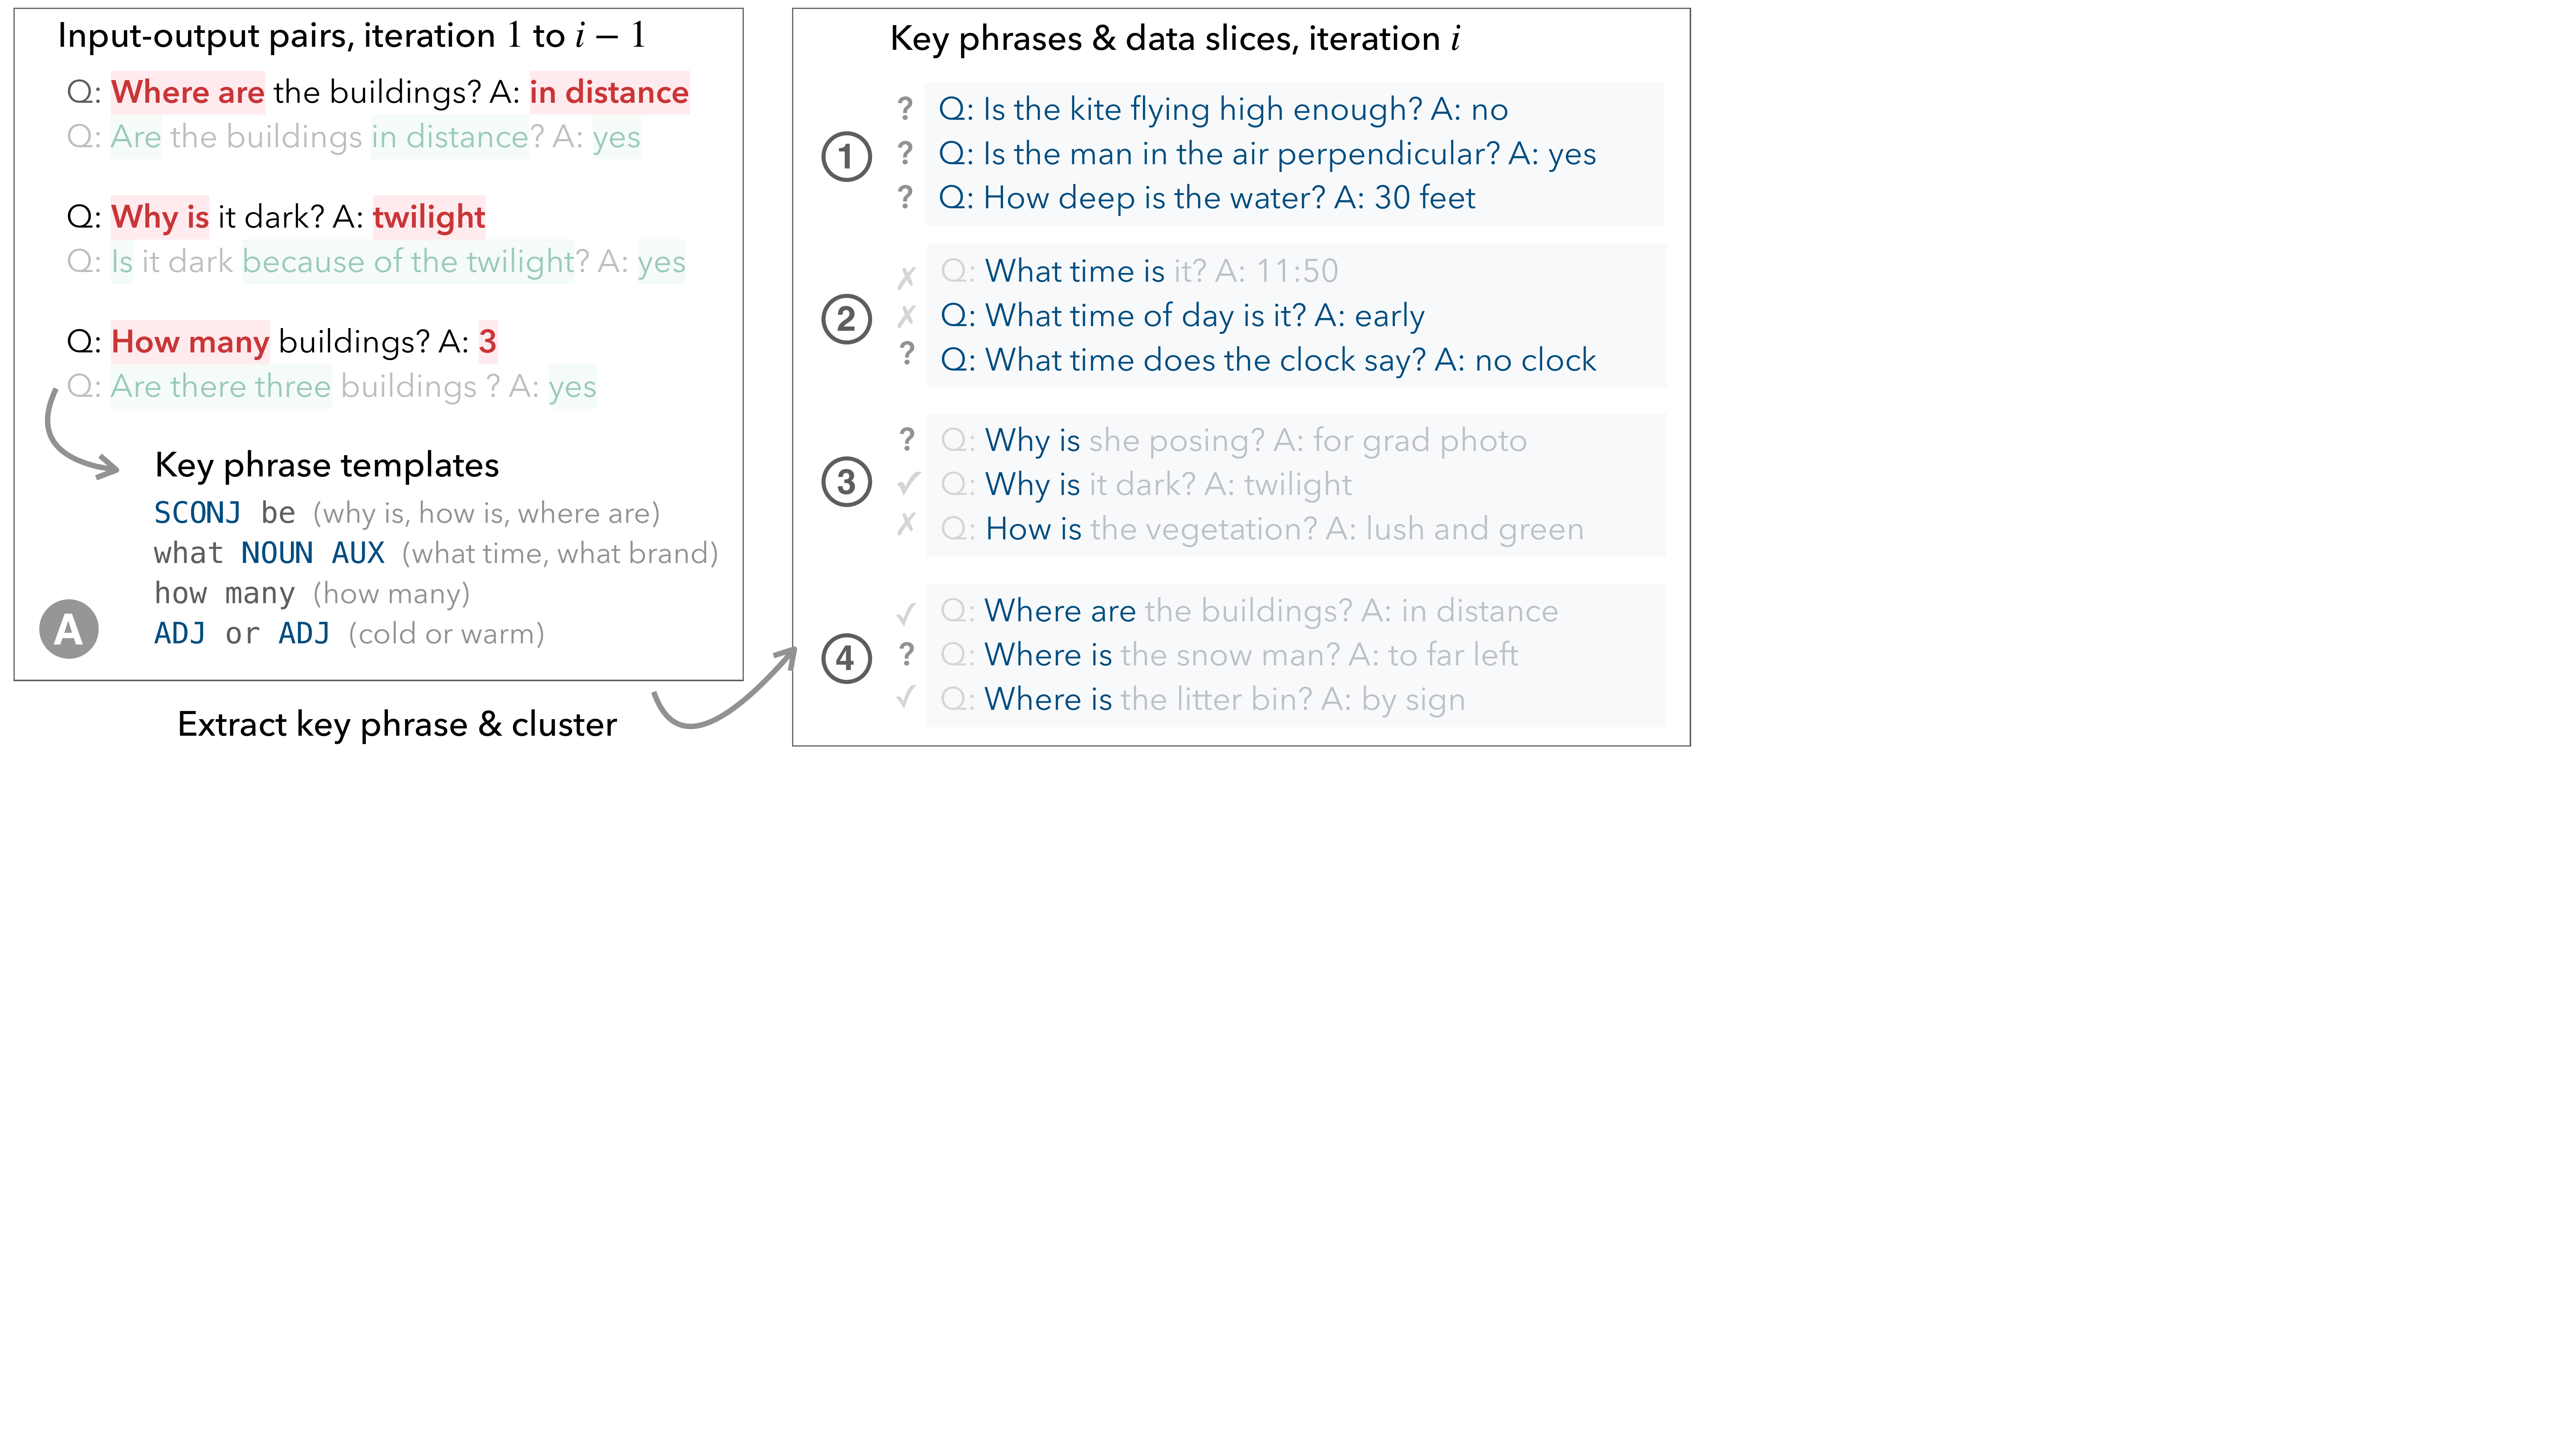}
\vspace{-15pt}
\caption{
A demonstration of the sampling procedure for \qa.
}
\vspace{-10pt}
\label{fig:slice_qa}
\end{figure*}
